# Supplementary material for: Hierarchical Graph Representation Learning with Differentiable Pooling
Source: arXiv:1806.08804 source file (2019-02-20)
Supplement: Supplementary file 1 [file 060appendix.tex]

\appendix

\section{Data Set Statistics}

The statistics of the data sets used in this paper are summarized in Table \ref{ds}.
\begin{table}[th!]
	\begin{center}
		\caption{Data set statistics and properties.}\label{dsstats}
		\resizebox{1.0\textwidth}{!}{ 	
			\begin{tabular}{@{}lccccc@{}}\toprule
				\multirow{3}{*}{\vspace*{4pt}\textbf{Data Set}}&\multicolumn{5}{c}{\textbf{Properties}}\\
				\cmidrule{2-6}
				&  Number of  Graphs & Number of Classes  &  Avg.\@ \# Nodes per Graph & Avg.\@ \# Edges per Graph & Node Labels \\ \midrule
				$\textsc{Collab}$ & 5000 & 3 & 74.49 & 2457.78 & \xmark \\
				$\textsc{D\&D}$ & 1178 & 2 & 284.32 & 715.66 & \cmark \\
				$\textsc{Enzymes}$ & 600 & 6 & 32.63 & 62.14 & \cmark \\
				$\textsc{Proteins}$ & 1113 & 2 & 39.06 & 72.82 &  \cmark \\
				$\textsc{Reddit-Multi-12k}$ & 11929 & 11 & 391.41 & 456.89 &  \xmark \\
				\bottomrule
			\end{tabular}}
			\label{ds}
		\end{center}
\end{table}

\section{Implementation Details}

\name is implemented using PyTorch, and tested on a machine with a TITAN Xp GPU. The input contains undirected graphs represented by adjacency matrices. We additionally use the degree, and the clustering coefficient as input feature for each node in the graphs.
When applying \name to \textsc{GraphSage}, the input adjacency matrices are not normalized, and bias terms are added to every graph convolutional layers.

In experiments, two sets of hyperparameters were used. For \textsc{Enzymes}, \textsc{Collab}, and \textsc{Proteins} data sets, the number of hidden dimensions is set to $64$. For \textsc{D\&D} and \textsc{Reddit-Multi-12k}, the number of hidden dimensions is set to $128$. The learning rate is chosen by a hyper-parameter sweep from $10^{-5}$ to $10^{-2}$.  In addition, the hidden representations at all layers are concatenated together to obtain the final graph representation.
After each layer of graph convolution, the embeddings are $\ell_2$-normalized, and a batch normalization layer is added. Empirically we find that adding the batch normalization layer helps alleviating the problem of overfitting.

We use a 2-layer perceptron (MLP) with ReLU non-linearity after the first layer and softmax after the second layer to map the graph representation to a vector of class probabilities. The cross entropy function is used to compute the loss. The hidden dimension of the MLP is equal to the hidden dimension of the GNN. 
To add the link prediction side objective, we first compute the Frobenius norm as detailed in the paper, and then normalize by the number of entries in the adjacency matrix.

Optimization is performed with the Adam optimizer, and the gradient is clipped when its norm is larger than $2.0$. The number of epochs trained is 4\,000, with early stopping when the average of validation loss in a moving window starts to decrease. 

\section{Extension to Graph Classification Tasks with Edge Features}

Although the datasets used for experiments do not contain features, \name could be extended to handle such cases.
A possible approach is to use a GNN similar to \cite{kipf2018neural}. Note that both the pooling and embedding network are flexible and models incorporating edge features can be applied.
However, note that in certain graphs with edge labels (e.g., molecule graphs), it could also be useful to modify the auxiliary link prediction objective to make it more consistent with the application.
For example, it is more meaningful to enforce that the clusters in a molecule are connected by small number of single bonds.
The corresponding auxiliary objective penalizes for the entry $(i,j)$ in cluster similarity matrix $S S^T$ that are close to $0$ (two nodes with different cluster assignment), if the edge $A_{i,j}$ is a non-single bond.
